# Supplementary material for: Structural evolution of amorphous polymeric nitrogen from \textit{ab initio} molecular dynamics simulations and evolutionary search
Source: arXiv:1804.09072 source file (2018-11-20)
Supplement: Supplementary file 1 [file Amorphous_Nitrogen_Supplemental.pdf]

# Supplemental material

## Radial distribution function restricted to atoms distant by $n$ bonds ($n$-th neighbours)

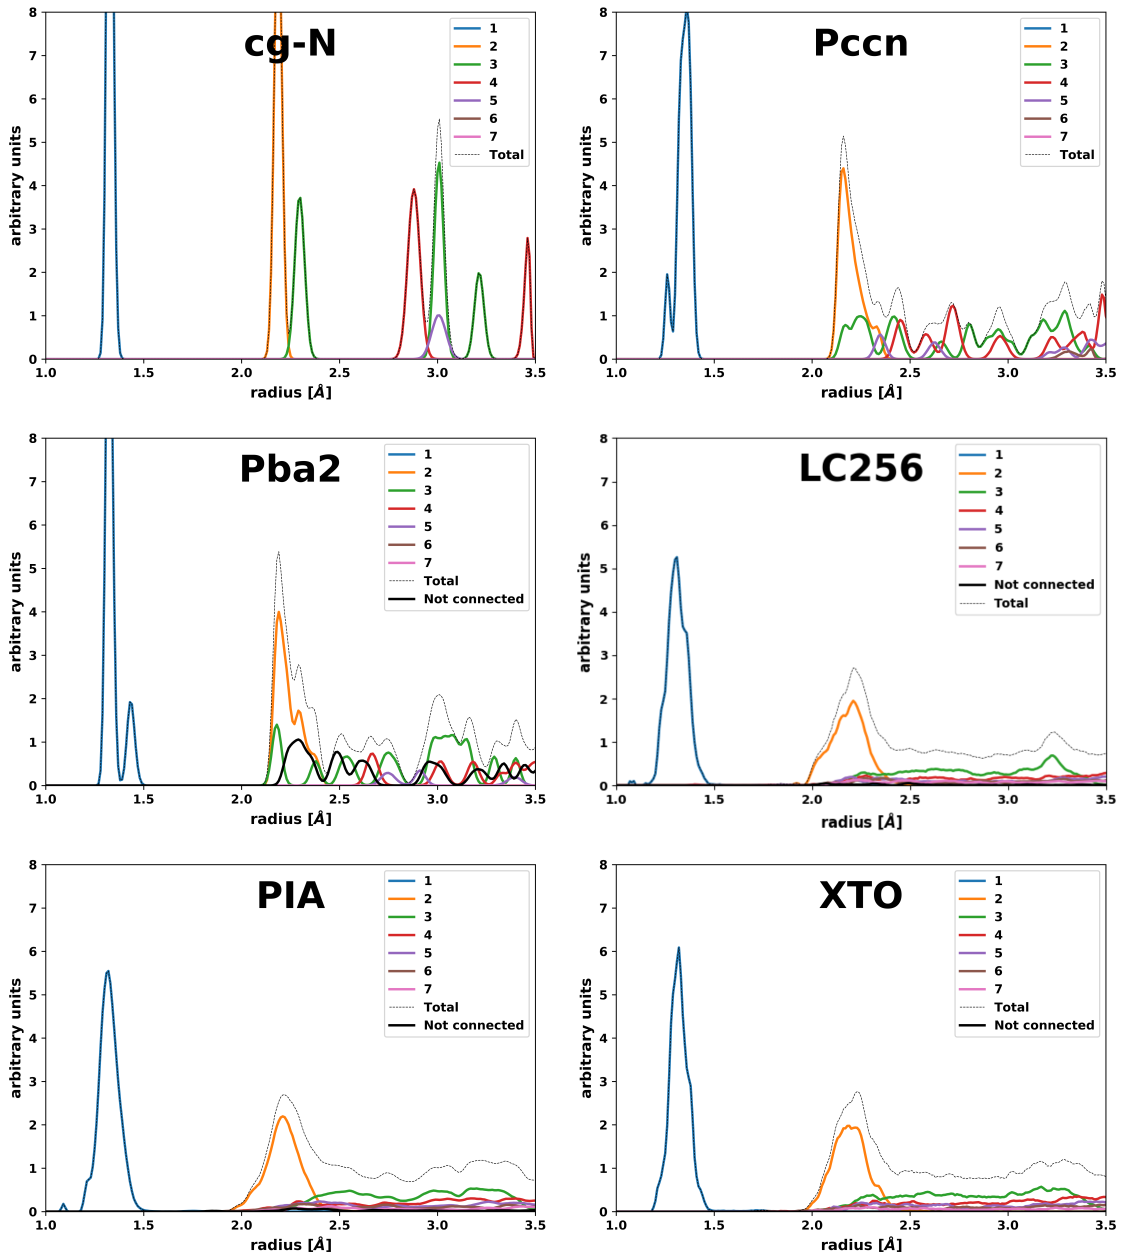


Figure 1: Radial distribution function restricted to atoms distant by $n$ bonds for various nitrogen phases at 120 GPa obtained from 1 ps MD at 100 K. The curves correspond to structures cg-N (top left), *Pccn* (top right), *Pba2* (center left), a-N (LC256) (center right), a-N (PIA) (bottom left) and a-N (XTO) (bottom right). We note that our amorphous structures have quite similar RDF even though they were prepared by three different ways. On the other hand, the RDF of crystalline cg-N structure is significantly different. This structure consists exclusively of rings with size of 10 atoms. The particular arrangement of rings results in some of the 4th neighbours being closer than most of 3rd neighbours. Interestingly the 5th neighbour (vis-à-vis atom in ring) has the same distance from reference atom as the second peak of 3rd neighbours. The presence of pronounced peaks between 2.7 and 3 $\AA$ makes RDF of cg-N unique and different from other crystalline polymeric nitrogen phases and a-N. The *Pccn* structure which can be considered as distorted cg-N structure with rings of length 8, 10 and 12, loses many of these features, making its RDF more similar to other RDFs. Layered *Pba2* has the most similar RDF to amorphous structures.

# Rings statistics histogram

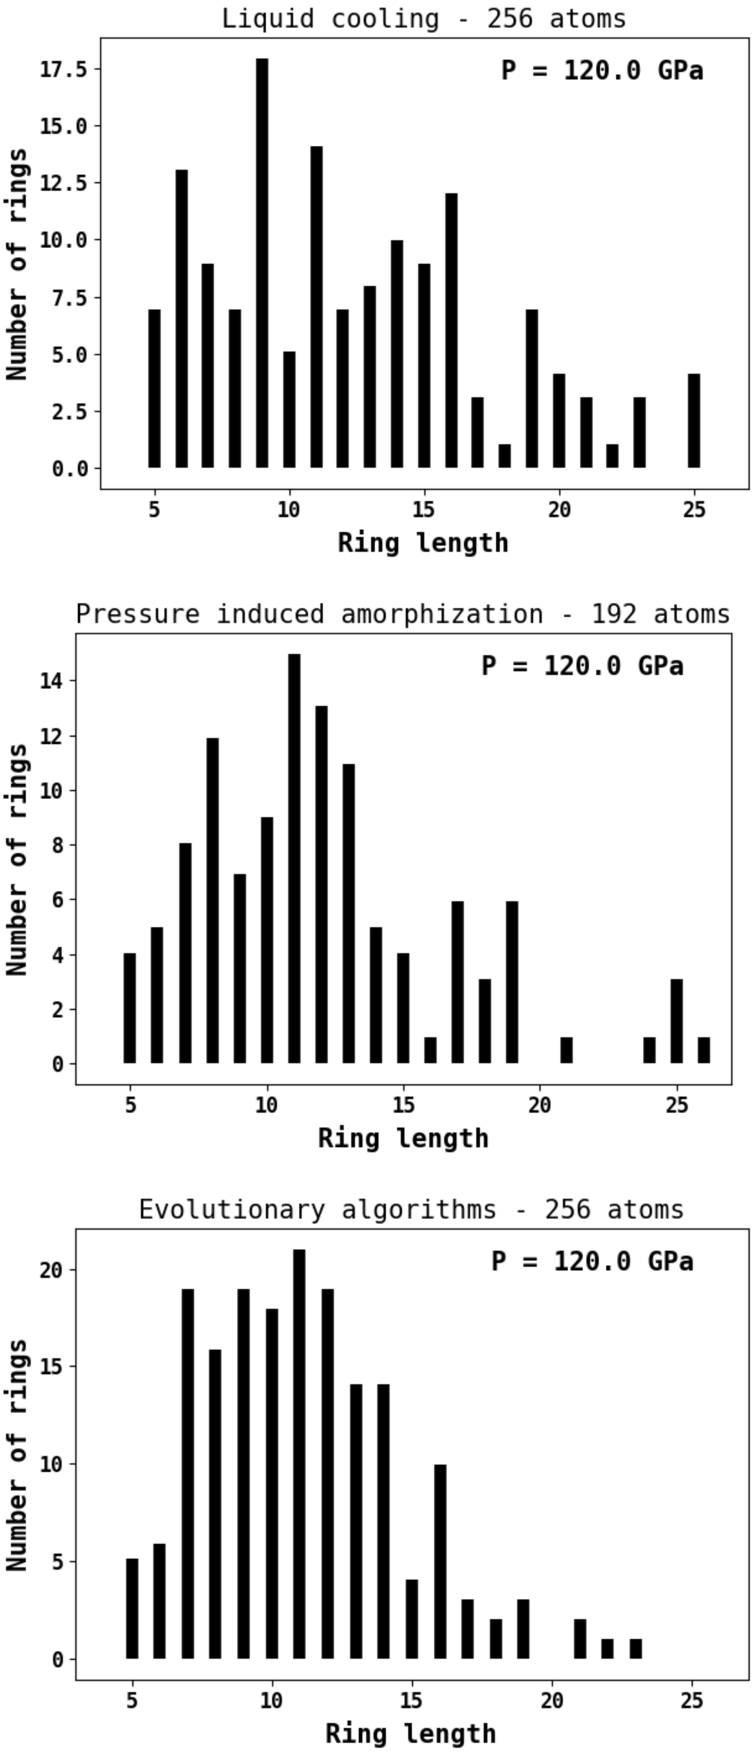


Figure 2: Rings statistics of a-N prepared by liquid cooling (top), pressure induced amorphization (middle) and evolutionary algorithms (bottom).

## Electronic density of states

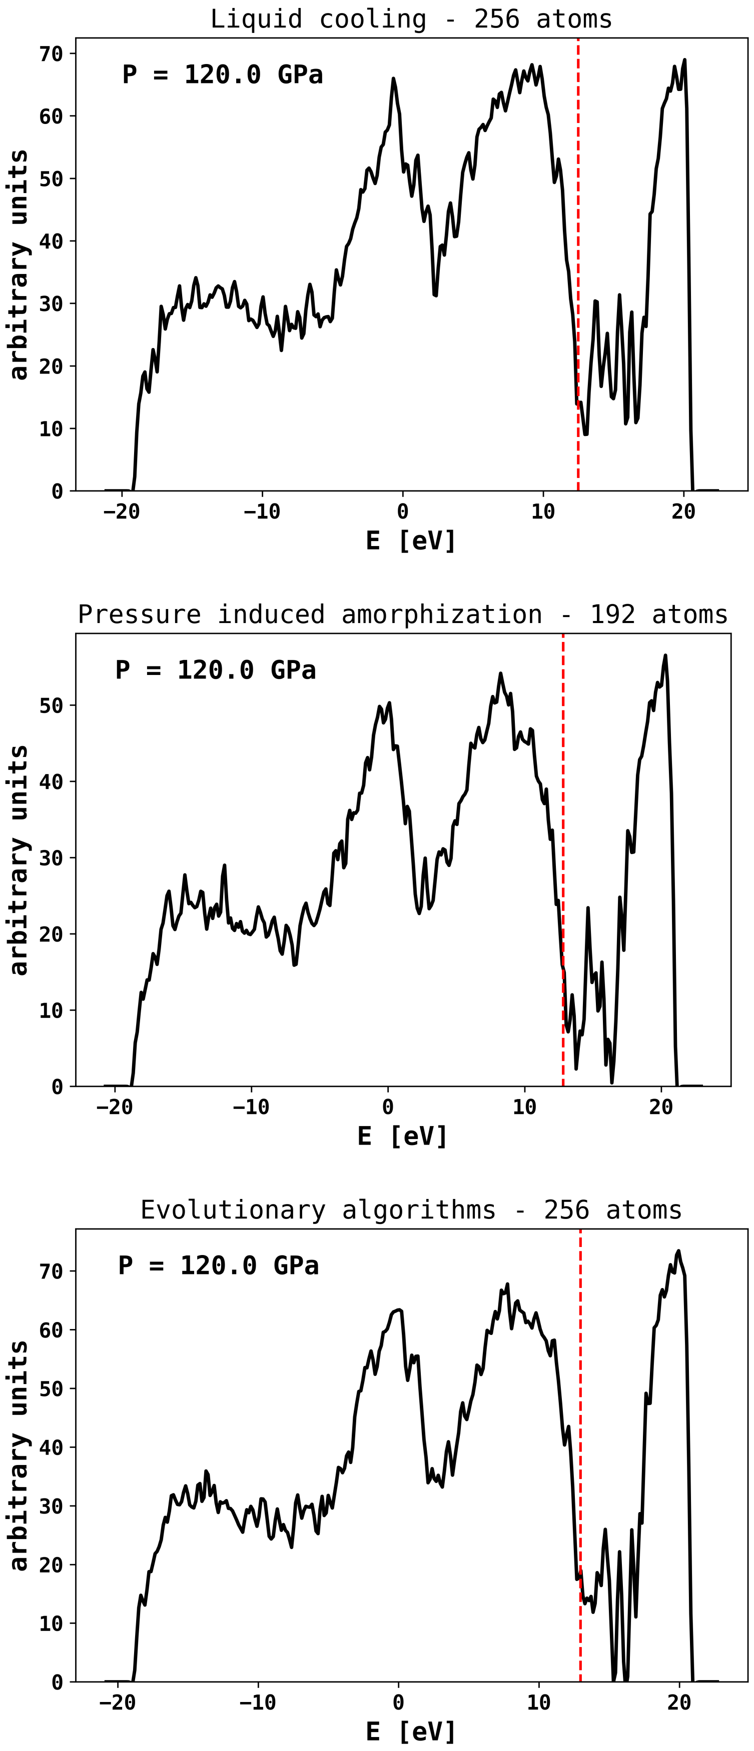


Figure 3: Electronic DOS (calculated with the SCAN functional) of a-N prepared by liquid cooling (top), pressure induced amorphization (middle) and evolutionary algorithms (bottom). Red dotted line represents the Fermi energy.
